# Supplementary material for: Extension of the Trotterized Unitary Coupled Cluster to Triple Excitations
Source: arXiv:2212.12462 ancillary file (2023-03-17)
Supplement: Supplementary file 1 [file Supplementary_Materials-UCCSDT.pdf]

# Supplementary Materials: Extension of the Trotterized Unitary Coupled Cluster to Triple Excitations


Mohammad Haidar,[†,‡,¶] M. J. Rančić,[¶] Y. Maday,[‡,§] and J-P. Piquemal[*,†]

†*Sorbonne Université, Laboratoire de Chimie Théorique(UMR-7616-CNRS), 4 place Jussieu-75005 Paris, France*

‡*Sorbonne Université, CNRS, Université Paris Cité, Laboratoire Jacques Louis Lions (LJLL), 4 place Jussieu-75005 Paris, France*

¶*TotalEnergies, Tour Coupole La Défense, 2 Pl. Jean Millier, 92078 Paris, France*

§*Institut Universitaire de France, Paris, France*

E-mail: Mohammadhaidar2016@outlook.com,jean-philip.piquemal@sorbonne-universite.fr

**Algorithm 1:** Implementation of the Triple Excitations (a similar algorithm for single and double excitations can be found in the code)

$n_{orb} \leftarrow$ Number of spin orbitals;
$n_{occ} \leftarrow$ Number of occupied orbitals;
$\hat{s}_e(\cdot, \cdot, \cdot) \leftarrow$ Orbital symmetry operator: A mapping between three orbitals and the product of their irreducible representations;
$L_3 \leftarrow$ Empty list;
**for** *each Unordered Triplet of Distinct Even Integers* $0 <= (i, j, k) < n_{occ}$ **do**
**for** *each Unordered Triplet of Distinct Even Integers* $n_{occ} <= (a, b, c) < n_{orb}$ **do**
**if** $\hat{s}_e(i, j, k) = \hat{s}_e(a, b, c)$ **then**
**Append** $(\hat{a}^\dagger_a \hat{a}^\dagger_b \hat{a}^\dagger_c \hat{a}_k \hat{a}_j \hat{a}_i - \hat{a}^\dagger_i \hat{a}^\dagger_j \hat{a}^\dagger_k \hat{a}_c \hat{a}_b \hat{a}_a)$ **to** $L_3$
**end**
**end**
**end**
**for** *each Unordered Triplet of Distinct Odd Integers* $0 <= (\bar{i}, \bar{j}, \bar{k}) < n_{occ}$ **do**
**for** *each Unordered Triplet of Distinct Odd Integers* $n_{occ} <= (\bar{a}, \bar{b}, \bar{c}) < n_{orb}$ **do**
**if** $\hat{s}_e(\bar{i}, \bar{j}, \bar{k}) = \hat{s}_e(\bar{a}, \bar{b}, \bar{c})$ **then**
**Append** $(\hat{a}^\dagger_{\bar{a}} \hat{a}^\dagger_{\bar{b}} \hat{a}^\dagger_{\bar{c}} \hat{a}_{\bar{k}} \hat{a}_{\bar{j}} \hat{a}_{\bar{i}} - \hat{a}^\dagger_{\bar{i}} \hat{a}^\dagger_{\bar{j}} \hat{a}^\dagger_{\bar{k}} \hat{a}_{\bar{c}} \hat{a}_{\bar{b}} \hat{a}_{\bar{a}})$ **to** $L_3$
**end**
**end**
**end**
**for** *each Unordered Pair of Distinct Even Integers* $0 <= (i, j) < n_{occ}$ **do**
**for** *each Unordered Pair of Distinct Even Integers* $n_{occ} <= (a, b) < n_{orb}$ **do**
**for** *each Odd Integer* $0 <= \bar{k} < n_{occ}$ **do**
**for** *each Odd Integer* $n_{occ} <= \bar{c} < n_{orb}$ **do**
**if** $\hat{s}_e(i, j, \bar{k}) = \hat{s}_e(a, b, \bar{c})$ **then**
**Append** $(\hat{a}^\dagger_a \hat{a}^\dagger_b \hat{a}^\dagger_{\bar{c}} \hat{a}_{\bar{k}} \hat{a}_j \hat{a}_i - \hat{a}^\dagger_i \hat{a}^\dagger_j \hat{a}^\dagger_{\bar{k}} \hat{a}_{\bar{c}} \hat{a}_b \hat{a}_a)$ **to** $L_3$
**end**
**end**
**end**
**end**
**end**
**for** *each Unordered Pair of Distinct Odd Integers* $0 <= (\bar{i}, \bar{j}) < n_{occ}$ **do**
**for** *each Unordered Pair of Distinct Odd Integers* $n_{occ} <= (\bar{a}, \bar{b}) < n_{orb}$ **do**
**for** *each Even Integer* $0 <= k < n_{occ}$ **do**
**for** *each Even Integer* $n_{occ} <= c < n_{orb}$ **do**
**if** $\hat{s}_e(\bar{i}, \bar{j}, k) = \hat{s}_e(\bar{a}, \bar{b}, c)$ **then**
**Append** $(\hat{a}^\dagger_{\bar{a}} \hat{a}^\dagger_{\bar{b}} \hat{a}^\dagger_c \hat{a}_k \hat{a}_{\bar{j}} \hat{a}_{\bar{i}} - \hat{a}^\dagger_{\bar{i}} \hat{a}^\dagger_{\bar{j}} \hat{a}^\dagger_k \hat{a}_c \hat{a}_{\bar{b}} \hat{a}_{\bar{a}})$ **to** $L_3$
**end**
**end**
**end**
**end**
**end**

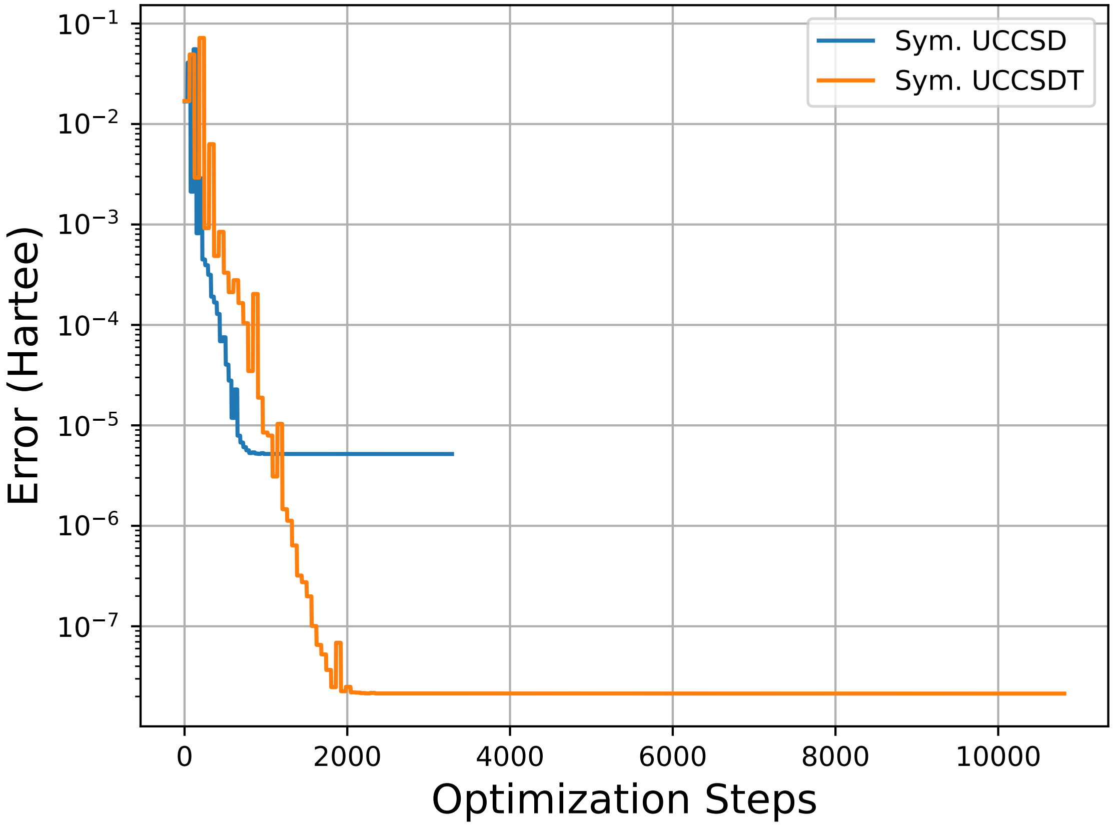


Figure 1: Convergence study of LiH at R = 1.0 Å using sym-UCCSD and -UCCSDT. BFGS optimizer: gradient Norm and energy change set at $10^{-10}$ Ha.

Table 1: Trotterization study of UCC-VQE simulations with different Trotter steps $t$ for LiH at various bond lengths: $R$ = 1.0 Å and $R$ = 3.0 Å. The obtained UCC-energies are in Hartree (Ha). The error (Err) is the difference between the estimated UCC-energy and the FCI.

| **Method** | | **R=1.0 Å** | | **R=3.0 Å** | |
|---|---|---|---|---|---|
| | | **Ener. (Ha)** | **Err. (Ha)** | **Ener. (Ha)** | **Err. (Ha)** |
| Trotter. (steps $t$) | 1-Sym.UCCSD | −7.78445509065 | $5.18 \times 10^{-6}$ | −7.79875240726 | $9.07 \times 10^{-5}$ |
| | 5-Sym.UCCSD | −7.78445509065 | $5.18 \times 10^{-6}$ | −7.79875240727 | $9.07 \times 10^{-5}$ |
| | 15-Sym.UCCSD | −7.78445509065 | $5.18 \times 10^{-6}$ | −7.79875240726 | $9.07 \times 10^{-5}$ |
| Trotter. (steps $t$) | 1-Sym.UCCSDT | −7.78446025863 | $2.13 \times 10^{-8}$ | −7.79884308642 | $7.30 \times 10^{-8}$ |
| | 2-Sym.UCCSDT | −7.78446025863 | $2.13 \times 10^{-8}$ | −7.79884308643 | $7.30 \times 10^{-8}$ |
| | 3-Sym.UCCSDT | −7.78446025863 | $2.13 \times 10^{-8}$ | −7.79884308644 | $7.30 \times 10^{-8}$ |

Table 2: Testing commutation of operators in UCC-VQE: The ratio of the commuting operators in the symmertic and non-symmetric ansatz, tested in LiH and $BeH_2$. This ratio is estimated by counting the number of all the possible commuting pairs divided by the total number of operators in the ansatz. The total number of operators is counted at different level of excitations as given in column 2.

| **Molecule (point group)** | **Excitation level** | **Percentage of commuting pairs (%)** | |
|---|---|---|---|
| | | **Symmetric Case** | **Non-Symmetric Case** |
| LiH ($C_{2v}$) | Single | 71.43 | 73.33 |
| | Single+Double | 24.42 | 21.31 |
| | Single+Double+Triple | 10.71 | 6.71 |
| $BeH_2$($D_{2h}$) | Single | 86.67 | 78.26 |
| | Single+Double | 33.14 | 30.08 |
| | Single+Double+Triple | 13.83 | 8.56 |

*

Table 3: Sym-UCCSD and sym-UCCSDT Total energies for LiH compared to FCI (STO-3G) and calculated in a range of bond lengths. The energy convergence is set to $10^{-10}$.

| R (Å) | Sym. UCCSD (Hartee) | Sym. UCCSDT (Hartee) | FCI (Hartee) |
|---|---|---|---|
| 0.5 | −7.0501644148779380 | −7.**05022**35647256120 | −7.0502250352999525 |
| 0.75 | −7.5754787130406010 | −7.**575486**6339520905 | −7.5754867198560570 |
| 1.0 | −7.7844550906578240 | −7.**7844602**586044880 | −7.7844602800312270 |
| 1.25 | −7.8618546821108560 | −7.**8618614**266821860 | −7.8618614405476190 |
| 1.5 | −7.8823528524099160 | −7.**8823622**687317640 | −7.8823622867987250 |
| 1.75 | −7.8771739864878560 | −7.**87718**69734608290 | −7.8771870023045400 |
| 2.0 | −7.8610690464555800 | −7.**86108772**93115270 | −7.8610877724814950 |
| 2.25 | −7.8417893122484820 | −7.**841817**7990484540 | −7.8418178594585280 |
| 2.5 | −7.8236791957091150 | −7.**8237238**068379700 | −7.8237238834676990 |
| 2.75 | −7.8090952255655415 | −7.**8091622**151773070 | −7.8091622976751710 |
| 3.0 | −7.7987524072724800 | −7.**798843**0864380140 | −7.7988431595024075 |
| 3.25 | −7.7920744784823260 | −7.**7921844**160797340 | −7.7921844720051410 |
| 3.5 | −7.7879918765157190 | −7.**788115**0827023810 | −7.7881151232808100 |

Table 4: Same information as in Table 4. However, for $BeH_2$ the point group is $D_{2h}$

| R (Å) | Sym. UCCSD (Hartee) | Sym. UCCSDT (Hartee) | FCI (Hartee) |
|---|---|---|---|
| 0.5 | −13.689363718754809 | −13.**6899**42413943600 | −13.689960305740938 |
| 0.75 | −15.038389733024509 | −15.**0387**14523994160 | −15.038723029097564 |
| 1.0 | −15.481475219860556 | −15.**4817**34432023574 | −15.481741069507574 |
| 1.25 | −15.591439321245653 | −15.**5917**61157486994 | −15.591770742728592 |
| 1.5 | −15.575474929852130 | −15.**5760**28912099567 | −15.576051245231916 |
| 1.75 | −15.514267857565354 | −15.**5154**22420566953 | −15.515486684790002 |
| 2.0 | −15.443240804842018 | −15.**4459**12543615990 | −15.446093740442993 |
| 2.25 | −15.380980950261227 | −15.**38**6994348454232 | −15.387444022410582 |
| 2.5 | −15.340092110289588 | −15.**33**8001074632515 | −15.336804236064943 |
| 2.75 | −15.322243062902645 | −15.**33**6971436621809 | −15.339271790108743 |
| 3.0 | −15.318390655555604 | −15.**35**0572088964430 | −15.351834313507846 |
| 3.25 | −15.321848064767805 | −15.**33**8080664477294 | −15.336613616187758 |
| 3.5 | −15.327893333570623 | −15.**33**5087260729638 | −15.336721455040767 |

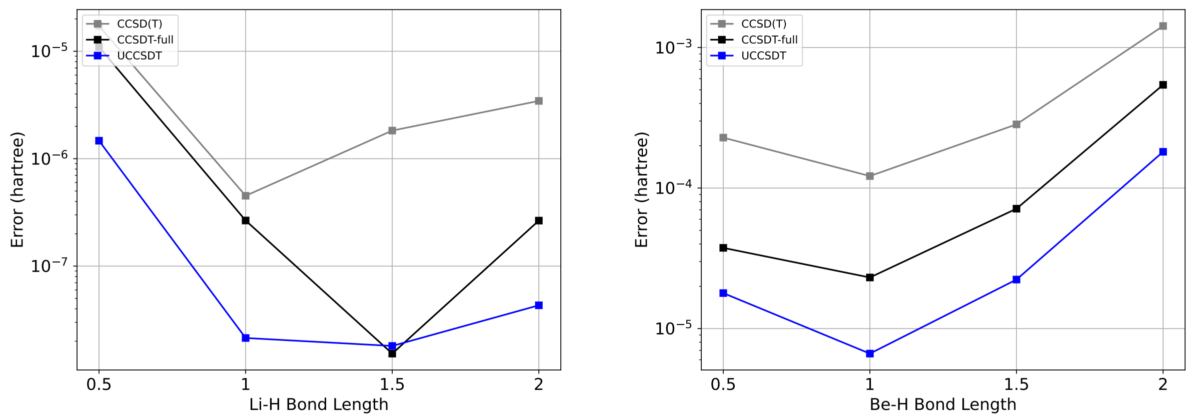


(a) LiH: Data of UCCSDT are from table 3. (b) $BeH_2$: Data of UCCSDT are from table 4.

Figure 2: Comparison of errors between Sym-UCCSDT, CCSD(T) and CCSDT-full. The Error represent the difference between Total energies and FCI(STO-3G). Data of CCSD(T) and CCSDT-full are taken from Table 5.

Table 5: CCSD, CCSD(T) and CCSDT-full Total Energies for LiH, $BeH_2$ and $H_2O$ using the STO-3G basis set. The second column represents the geometry of the three molecules. Note that those dented by (Equi) are the geometric data found in the CCCBDB-NIST Database.[1]

| Molecule | Geometry | CCSD (Hartee) | CCSD(T) (Hartee) | CCSDT-full (Hartee) |
|---|---|---|---|---|
| LiH | Equi | −7.882392916908374 | −7.8824013049480515 | −7.882403382419276 |
| | $R$ = 0.5Å | −7.0501599111782935 | −7.0502078462630395 | −7.0502140845154420 |
| | 1.0Å | −7.7844548259108270 | −7.7844598283190605 | −7.7844605459246266 |
| | 1.5Å | −7.8823529091527020 | −7.8823604602026290 | −7.8823623021310300 |
| | 2.0Å | −7.8610699254312260 | −7.8610843221359294 | −7.8610875072227335 |
| $BeH_2$ | Equi | −15.59478311558745 | −15.59499296964964 | −15.595134697924136 |
| | 0.5 | −13.689341503735706 | −13.689731786245128 | −13.689922761413788 |
| | 1.0Å | −15.481463481056172 | −15.481619345311978 | −15.481717966125348 |
| | 1.5Å | −15.575461402861198 | −15.575767243189018 | −15.575979921679428 |
| | 2.0Å | −15.443247546742555 | −15.444670661700785 | −15.445551002948804 |
| $H_2O$ | Equi | −75.01246171279932 | −75.01252912274785 | −75.01255654380829 |

# References

(1) Lovas, F.; Tiemann, E.; Coursey, J.; Kotochigova, S.; Chang, J.; Olsen, K.; Dragoset, R. Diatomic Spectral Database. https://www.nist.gov/pml/diatomic-spectral-databaseDiatomic spectral database, 2003.
